# Supplementary material for: Unraveling the reaction mechanisms leading to partial fusion of weakly bound nuclei
Source: arXiv:1910.06625 source file (2019-10-15)
Supplement: Supplementary file 1 [file supplemental.pdf]

# Supplemental material for "Unraveling the reaction mechanisms leading to partial fusion of weakly bound nuclei"

Jin Lei[1,*] and Antonio M. Moro[2,†]

[1]Institute of Nuclear and Particle Physics, and Department of Physics and Astronomy, Ohio University, Athens, Ohio 45701, USA

[2]Departamento de FAMN, Universidad de Sevilla, Apartado 1065, 41080 Sevilla, Spain.

## I. EXPLICIT CONTRIBUTION BREAKUP-FUSION MECHANISM

In Figs. 2 and 3 of the Letter, we show the predictions for non-elastic breakup (NEB) cross sections for the $^{93}$Nb($d$,$pX$) and $^{209}$Bi($^6$Li,$\alpha X$) reactions obtained with Eq. (3), but retaining only the ground-state (g.s.) part of the CDCC function in the computation of the channel wavefunction $\varphi_x$ [c.f. Eqs. (4) and (5)]. In both cases, this calculation, denoted IAV-CDCC(gs), turns out to be very close to the full IAV-CDCC result, in which the full CDCC wavefunction is considered in the computation of $\varphi_x$. Although this result clearly indicates that the BF mechanism is very small in both reactions, we cannot completely rule out some cancellation between the continuum contribution to $\varphi_x$ and the interference terms between the ground-state and continuum parts in Eq. (3).

To pin down the importance of the unbound components of the CDCC wavefunction, Eq. (5) on the NEB cross sections (and hence assess the importance of these interference terms) we present here additional calculations for these two reactions, including only the continuum part of the CDCC wavefunction (5) in the evaluation of Eq. (3). The results are shown in Fig. 1 and Fig. 2 of this document. It can be seen that this contribution is negligibly small and, hence, the interference term must be also very small.

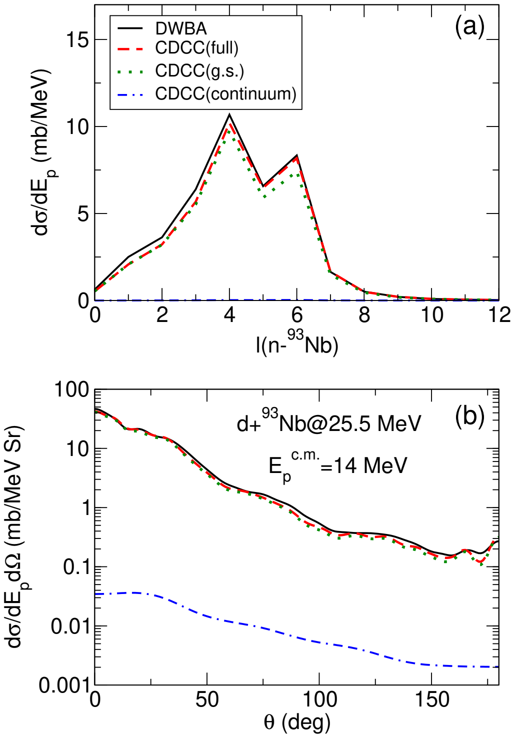


FIG. 1. Non-elastic breakup contribution for the reaction for $^{93}$Nb($d$,$p$X) at $E_{\rm lab} = 25.5$ MeV for an outgoing proton C.M. energy of 14 MeV. (a) Energy differential cross section as a function of the neutron-target orbital angular. (b) Double differential cross section angular distribution.

## II. NON-ELASTIC BREAKUP *VERSUS* INCOMPLETE-FUSION

Although the main focus of our paper is the understanding of the nature of the incomplete-fusion (ICF) mechanism, our calculations provide the full non-elastic breakup (NEB) contribution which, in addition to ICF, includes other possible channels, such as projectile breakup accompanied by target excitation.

Since ICF is known to be the major contributor of NEB, one expects that the conclusions drawn for the NEB part will remain for the ICF part. In this document we provide a more quantitative support for this statement. For that, we resort to the idea that the ICF part can be identified with the absorption originated by the inner part of the $x-A$ interaction $W_{xA}$ whereas other contributors associated with direct reactions of $x$ with $A$, such as the projectile dissociation concomitant with target excitation, will have a more peripheral nature. This suggests an approximate procedure of separating the ICF from other NEB contributions consisting in splitting the imaginary part $W_{xA}$ into two parts $W_{xA} = W_{xA}^{CN} + W_{xA}^{\rm DR}$,

* jinl@ohio.edu
† moro@us.es

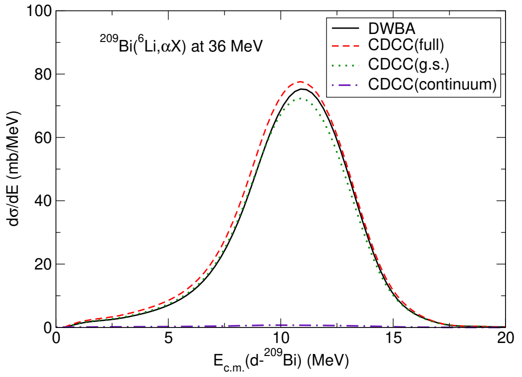


FIG. 2. NEB differential cross sections for the $^{209}$Bi($^6$Li,$\alpha X$) reaction at 36 MeV as a function of the $d$-$^{209}$Bi relative energy. The IAV-DWBA calculation (black solid line) is compared with the full IAV-CDCC calculation (red dashed line) and with truncated IAV-CDCC calculations using only the ground-state contribution of the CDCC wavefunction (dotted) or its continuum contribution (dot-dashed).

with $W^{CN}_{xA}$ and $W^{\rm DR}_{xA}$ representing the inner and peripheral parts, associated, respectively, with the compound nucleus (ICF) and direct reactions (DR) processes [1–3]. Thus, one can estimate the ICF contribution as

$$\left.\frac{d^2\sigma}{dE_b d\Omega_b}\right|_{\rm ICF} = -\frac{2}{\hbar v_a}\rho_b(E_b)\langle\varphi_x(\mathbf{k}_b)|W^{CN}_{xA}|\varphi_x(\mathbf{k}_b)\rangle, \tag{1}$$

A difficulty of this procedure is the ambiguity associated with the choice of $W^{CN}_{xA}$ and $W^{\rm DR}_{xA}$. For the present purposes, we can nevertheless get an idea of the relative importance of the inner and peripheral parts by inspecting the quantity $|\varphi_x(r_x)|^2\ W_{xA}(r_x)\ r_x^2$ (that is, the integrand of Eq. (3) of the paper) as a function of the $x-A$ distance. This is shown in Fig. 3 for the $^{93}$Nb(d,px) reaction at 25.5 MeV. Panels (a) and (b) display the modulus of the radial part of the channel function $\varphi_x$ as a function of the $x-A$ separation, computed either with the ground state part of the CDCC function or with the continuum *bins*, respectively. For concreteness, the configuration $\ell_x = \ell_b = 0$ has been considered, where $\ell_x$ and $\ell_b$ denote the angular momentum associated to the $x-A$ relative motion and $b-B$ relative motion, respectively. For the continuum states, only the $s$ ($l_{bx} = 0$) and $d$-waves ($l_{bx} = 2$)) are shown for simplicity. These results show the dominance of the projectile ground-state component in the $x-A$ wavefunction. This, in turn, results in a dominance of the IAV-CDCC(gs) in the NEB cross section, as can be verified in panels (c) and (d), where we display the quantity $|\varphi_x(r_x)|^2\ W_{xA}(r_x)\ r_x^2$ for the two choices of $\varphi_x$. As expected, it is seen that IAV-CDCC(gs) gives the dominant contribution in the whole radial range. Thus, if we associate $W^{CN}_{xA}$ with the contribution of $W^{CN}$ below a certain *fusion radius*, the dominance of the ground-state part will prevail for the ICF cross sections.

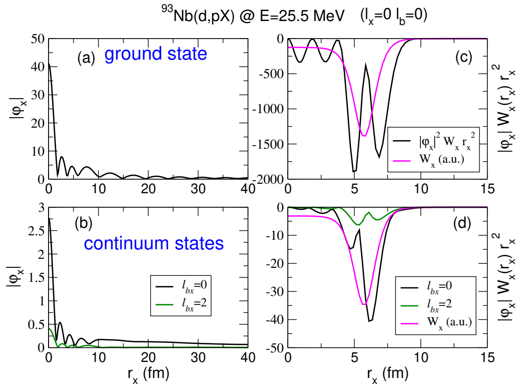


FIG. 3. Panels (a) and (b): Radial part of the channel wavefunction $\varphi_x(r_x)$ for the reaction $^{93}$Nb($d$,$p$x) at 25.5 MeV for, respectively, the ground state and continuum parts of the CDCC wavefunction used in the source term of Eq. (4). Panels (c) and (d): $|\varphi_x|^2 W_x(r_x) r_x^2$ considering the ground-state or continuum parts of of the CDCC wavefunction. For the continuum states, only the contributions from $s$ and $d$ waves are shown.


[1] R. Mastroleo, T. Udagawa, and M. Mustafa, Physical Review C **42**, 683 (1990).
[2] T. Udagawa, B. T. Kim, and T. Tamura, Phys. Rev. C **32**, 124 (1985).
[3] C. Bertulani, M. Hussein, and S. Typel, Physics Letters B **776**, 217 (2018).
